# Supplementary material for: Transport in strained graphene: Interplay of Abelian and axial magnetic fields
Source: arXiv:2212.00788 ancillary file (2023-11-02)
Supplement: Supplementary file 1 [file supplemental.pdf]

# Supplemental Material: Transport in strained graphene: Interplay of Abelian and axial magnetic fields

Aqeel Ahmed,[1, 2, *] Sanjib Kumar Das,[2, *] and Bitan Roy[2]

[1] *Department of Physics and Astronomy, Union College. Schenectady, NY, USA*
[2] *Department of Physics, Lehigh University, Bethlehem, Pennsylvania, 18015, USA*
(Dated: December 1, 2022)

In this Supplemental Material, (a) we present the additional details for derivation of the Peierls flux in presence of an orbital magnetic field. [Sec. S1], (b) evolution of the Landau levels (LLs) with varying relative strength of the Abelian ($B$) and axial ($b$) magnetic fields [Sec. S2], and (c) Four-terminal Hall conductivity calculation for the limit where strain field ($b$) dominates over the orbital magnetic field ($B$) [Sec. S3].

## S1. DERIVATION OF THE PEIERLS PHASE

In this section, we present the derivation of the Peierls phase in presence of an orbital magnetic field, which is presented in Eq. (2) of the main manuscript. The formula for calculating the Peierls phase reads

$$\phi_{jk} = \frac{e}{hc}\int_j^k \mathbf{A}\cdot\mathbf{dl}. \tag{S1}$$

Now, committing to the Landau gauge choice of $\mathbf{A} = (-By, 0, 0)$, we can parametrize the curve over which the line integral [Eq. (S1)] is to be performed with

$$\phi_{jk} = \int_0^1 \mathbf{A}(\mathbf{r}(\tau))\cdot\mathbf{r}'(\tau)d\tau, \tag{S2}$$

where, $\mathbf{A}$ is the vector field and the path is defined as $\mathbf{r}(\tau) = (1-\tau)(x_j, y_j) + \tau(x_k, y_k)$ with $0 \le \tau \le 1$. Note that setting $\tau = 0$, we obtain the initial point $(x_j, y_j)$ of the hopping bond, while $\tau = 1$ sets the final point $(x_k, y_k)$ of the path. With this we can define $\mathbf{r}'(\tau) = (-x_j + x_k, -y_j + y_k)$, and $\mathbf{A}(\mathbf{r}(\tau)) = -B(y_j - \tau y_j + \tau y_k)\hat{i}$. Taking the scalar product with the $\mathbf{r}'(\tau)$, we get $\mathbf{A}(\mathbf{r}(\tau))\cdot\mathbf{r}'(\tau) = -B(y_j - \tau y_j + \tau y_k)(-x_j + x_k)$. Thus, the Peierls phase can be written as

$$\phi_{jk} = -\frac{eB}{hc}\int_0^1 (y_j - \tau y_j + \tau y_k)(x_k - x_j)d\tau. \tag{S3}$$

On simplifying, we obtain $\phi_{jk} = -\frac{eB}{2hc}(y_j + y_k)(x_k - x_j)$. Plugging this value of the phase in $\exp(2\pi i\phi_{jk})$ yields $t \to te^{-i\pi B}(y_j + y_k)(x_k - x_j)$ as mentioned in the main manuscript. We set $e = h = c = 1$ for all our calculations.

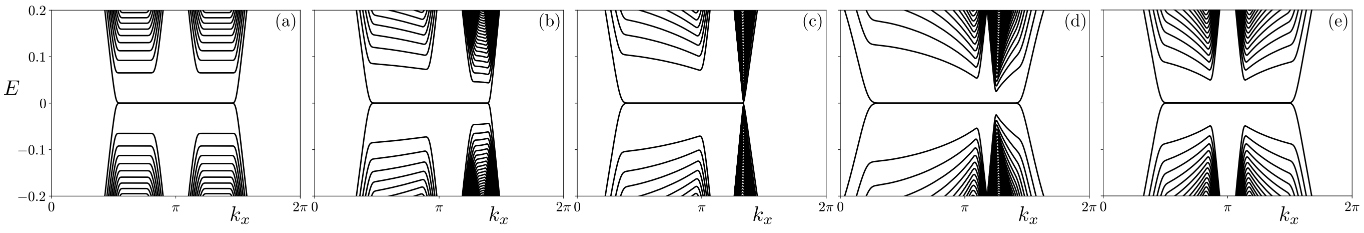


Figure S1. Band structures are depicted for (a) only Abelian magnetic field with $B = 4.5\times10^{-4}, \omega = 0$, (b) Abelian magnetic field dominated ($B = 4.5\times10^{-4}$) but with small strain field $\omega = 0.5$, (c) the quantum critical point $B = 4.5\times10^{-4}, \omega = 1.0$, (d) the strain field dominating over the Abelian field $B = 4.5\times10^{-4}, \omega = 1.6$, and (e) only strain limit with $B = 0, \omega = 1.25$. The zigzag graphene nanoribbon here contains 400 sites.

---

* Equal contributors.

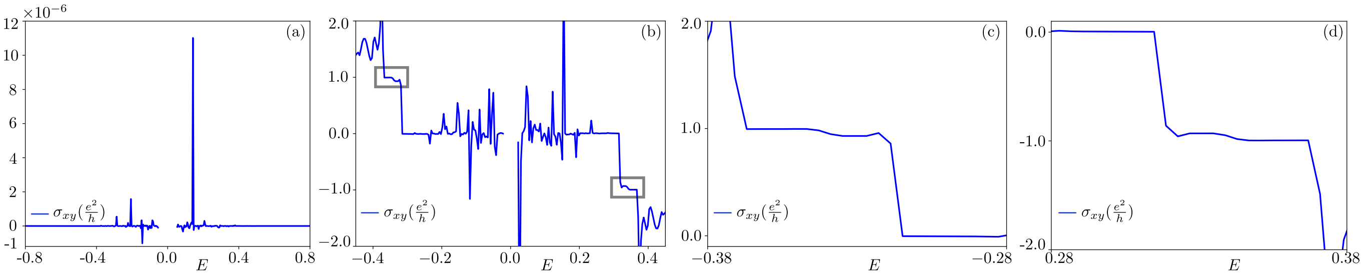


Figure S2. (a) Four-terminal Hall conductivity $\sigma_{xy}$ for $B = 0$ but $\omega = 0.3$, computed in a system of $L = W = 200$, showing that $\sigma_{xy} = 0$ within the numerical accuracy. (b) Four-terminal Hall conductivity is shown for $b > B$ with $B = 2\times10^{-5}, \omega = 0.3, \delta = 0$ in a system with $L = W = 600$. (c) and (d) are the zoomed in sections of the rectangular region marked in (b), displaying the quantized plateaus at $\sigma_{xy} = \pm 1$, respectively. The disconnected region in conductivity near the $E = 0$ occurs due to the finite size effects.

## S2. EVOLUTION OF THE LLS WITH VARYING RELATIVE STRENGTH OF $B$ AND $b$

In this section, we briefly discuss the evolution of the LLs in the presence of the Abelian ($B$) and axial ($b$) magnetic fields. The results are shown in Fig. S1. Notice that when $B \approx b$, one of the Dirac points becomes gapless, while the other one continues to host LLs. See Fig. S1(c). As mentioned in the main manuscript that it is challenging to extract $b$ in terms of the strain functions $\omega$ directly. However, the strength of $b$ can be pinned by identifying the quantum critical point, where one of the Dirac points becomes gapless for $B = b$, as we have precise measure of the strength of the Abelian magnetic field $B$.

## S3. FOUR-TERMINAL HALL CONDUCTIVITY FOR $b > B$

In this section, we present the four terminal transport results for the limit $b > B$, meaning when the pseudo magnetic field dominates over the orbital magnetic field. When we set $B = 0$, the Hall conductivity $\sigma_{xy} = 0$ within the numerical accuracy [Fig. S2(a)]. When $b > B$ and $B$ is finite, we notice that the Hall conductivity is numerically unstable throughout a large region upon changing the energy of the system [Fig. S2(b)]. Nevertheless, $\sigma_{xy}$ still shows integer plateaus at 1 and $-1$ near the first LL energies, as shown in Fig. S2(c) and (d), respectively.
